# Supplementary material for: Order Acquisition Under Competitive Pressure: A Rapidly Adaptive Reinforcement Learning Approach for Ride-Hailing Subsidy Strategies
Source: arXiv:2507.02244 source file (2025-07-04)
Supplement: Supplementary file 2 [file Appendix.pdf]

# Appendix of submission-1131

No Author Given

No Institute Given

## A Model Details

### A.1 Backbone Model Detail

In our study, we employ a logistic regression model to estimate the In-Range default selection probability, denoted as  $w_{ij}^{(in)}$ , and the In-Range completion probability, denoted as  $f_{ij}^{(in)}$ . The logistic model is formulated as  $Logistic(x, t) = C \cdot \sigma(W_1 x + b_1) \cdot t + (W_2 x + b_2)$ , where  $t$  represents the treatment variable,  $x$  is the input feature vector,  $\sigma(\cdot)$  is the sigmoid activation function,  $C$  is a scaling constant, and  $W_i, b_i$  are the model parameters. Additionally, we utilize a two-layer multilayer perceptron (MLP) to predict the two parameters of the beta distribution. All models are trained using a learning rate of 0.02, over 50 epochs, and optimized with the Adam optimizer in our experiments.

As depicted in Table 1, an increase in competitive behavior correlates with a decline in the predictive performance of the trained model, as evidenced by a reduction in the Area Under the Curve (AUC) metric. This suggests that heightened competition adversely affects the model’s ability to accurately predict outcomes.

## B Dataset Detail

The pre-training dataset is designed to include 168 slots, each simulating one hour within a day. The training dataset comprises 720 slots, while the test datasets consist of 336 slots. Each slot, representing a 24-hour period, encompasses a total of 40,000 orders. This structure allows for a comprehensive analysis of order patterns and behaviors over a simulated daily cycle.

As illustrated in Figure 1 and Table 2, the frequency of competitive behavior increases from Scene-1 to Scene-3. Scene-4, however, represents a stable environment characterized by minimal price change activity.

## C Formalization Proofs

In this section, we first derive the dual problem corresponding to the primal problem and then demonstrate that the optimal objective values of the primal and dual problems coincide. The optimal solution will be derived to the relaxed problem in the end.

Table 1: Backbone Model Performance

|         | Target          | Test AUC |
|---------|-----------------|----------|
| Scene-1 | $f_{ij}^{(in)}$ | 76.18    |
|         | $w_{ij}$        | 90.47    |
|         | $z_{ij}$        | 79.10    |
| Scene-2 | $f_{ij}^{(in)}$ | 79.78    |
|         | $w_{ij}$        | 88.83    |
|         | $z_{ij}$        | 81.88    |
| Scene-3 | $f_{ij}^{(in)}$ | 77.24    |
|         | $w_{ij}$        | 88.39    |
|         | $z_{ij}$        | 79.91    |
| Scene-4 | $f_{ij}^{(in)}$ | 76.48    |
|         | $w_{ij}$        | 91.42    |
|         | $z_{ij}$        | 77.79    |

Table 2: Dataset Configuration Table

| Scene-1                | Scene-2 | Scene-3 | Scene-4 |
|------------------------|---------|---------|---------|
| Change Probability 0.1 | 0.2     | 0.4     | 0.02    |

### C.1 Dual Problem

To derive the dual problem, we begin by relaxing the integer constraints on variables  $v_{ij} \in \{0, 1\}$  to continuous. Consequently, the optimization problem becomes:

$$\begin{aligned}
\min f_0(\mathbf{v}) &\triangleq - \sum_{i=0}^{N-1} \sum_{j=0}^{H-1} z_{ij} v_{ij} \\
\text{subject to } f_1(\mathbf{v}) &\triangleq \sum_{i=0}^{N-1} \sum_{j=0}^{H-1} g_i z_{ij} v_{ij} d_j - \sum_{i=0}^{N-1} \sum_{j=0}^{H-1} g_i z_{ij} v_{ij} \cdot B \leq 0
\end{aligned} \tag{1}$$

The above optimization function can be convert to minimizing the function  $J(\mathbf{v})$ :

$$J(\mathbf{v}) \triangleq f_0(\mathbf{v}) + I[f_1(\mathbf{v})] \tag{2}$$

where  $I[u] = 0$  if  $u \leq 0$  and  $I[u] = \infty$  otherwise. Define  $L(\mathbf{v}, \lambda) \triangleq f_0(\mathbf{v}) + \lambda f_1(\mathbf{v})$  and note that

$$J(\mathbf{v}) = \max_{\lambda \geq 0} L(\mathbf{v}, \lambda) \tag{3}$$

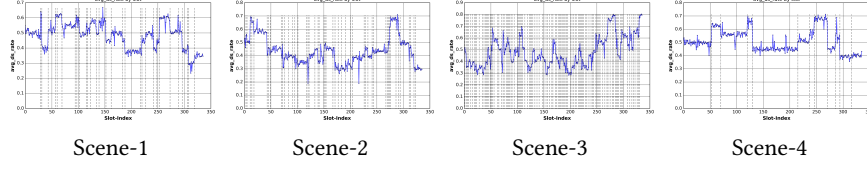

Fig. 1: IRR Rate for each Scene over each time step. The vertical dash line represents the slot point that the car partner changed prices.

This equation holds whether  $f_1(\mathbf{v})$  is non-positive or positive. If  $\mathbf{v}$  satisfies  $f_1(\mathbf{v}) \leq 0$ , then  $L(\mathbf{v}, \lambda)$  is maximized when taking  $\lambda = 0$ , and then  $L(\mathbf{v}, \lambda) = f(\mathbf{v}) = J(\mathbf{v})$ ; if  $\mathbf{v}$  violates constraint,  $f_1(\mathbf{v}) > 0$ , then  $L(\mathbf{v}, \lambda) \rightarrow \infty$  when  $\lambda \rightarrow \infty$ . Therefore, the original problem is equivalent to:

$$\min_{\mathbf{v}} \max_{\lambda \geq 0} L(\mathbf{v}, \lambda) \quad (4)$$

By reversing the order of  $\min$  and  $\max$ , we get

$$\max_{\lambda \geq 0} \min_{\mathbf{v}} L(\mathbf{v}, \lambda) = \sum_{i=0}^{N-1} \sum_{j=0}^{H-1} z_{ij} (\lambda g_i d_j - \lambda g_i B - 1) v_{ij} \quad (5)$$

This expression represents the dual formulation of the original problem.

## C.2 Strong Duality

The optimization problem satisfies the sufficient conditions for strong duality:

1. The goal function  $f_0(\cdot)$  and the constraint function  $f_1(\cdot)$  are both linear in  $\mathbf{v}$ , and hence, both are convex functions. Therefore, the problem is a convex optimization problem.
2. For any value of  $B > 0$ , there always exists  $v_{ij}$  small enough for any nonzero discounts  $d_j$  such that the strict inequality

$$f_1(\mathbf{v}) = \sum_{i=0}^{N-1} \sum_{j=0}^{H-1} g_i z_{ij} v_{ij} d_j - \sum_{i=0}^{N-1} \sum_{j=0}^{H-1} g_i z_{ij} v_{ij} \cdot B < 0$$

holds. In practice,  $B$  is usually large for a marketing campaign. This guarantees that the interior of the feasible region is non-empty.

Given that both the objective and constraint functions are convex, and that the problem satisfies the Slater condition, the original problem 1 and the dual problem 6 have strong duality. This duality ensures that the optimal objective values of the primal and dual problems are equal.

### C.3 Optimal Decision Function

Let us analyze the relaxed optimization function, as shown in Eq. 6. Given a fixed  $\lambda$ ,

$$\min_{\mathbf{v}} L(\mathbf{v}, \lambda) = \sum_{i=0}^{N-1} \min_{\mathbf{v}_i} \left[ \sum_{j=0}^{H-1} z_{ij} (\lambda g_i d_j - \lambda g_i B - 1) v_{ij} \right] \quad (6)$$

For each ride-hailing opportunity  $i$ , the items in  $L(\mathbf{v}, \lambda)$  associated with  $i$  consist of  $\sum_{j=0}^{H-1} z_{ij} (\lambda g_i d_j - \lambda g_i B - 1) v_{ij}$ . Now, we reintroduce the constraints  $\sum_{j=0}^{H-1} v_{ij} - 1 = 0$  and  $v_{ij} \geq 0$  to the problem. Thus, for a fixed  $\lambda$ , the original minimization problem can be decomposed into  $N$  sub-optimization problems, for each  $i \in \{0, 1, \dots, N-1\}$ , the problem is:

$$\begin{aligned} \min h(\mathbf{v}_i) &\triangleq \sum_{j=0}^{H-1} z_{ij} (\lambda g_i d_j - \lambda g_i B - 1) v_{ij} \\ \text{subject to } &\sum_{j=0}^{H-1} v_{ij} = 1, v_{ij} \geq 0 \end{aligned} \quad (7)$$

The optimal solution to this problem can be easily obtained using a greedy algorithm. Specifically, its optimal value is

$$j^* = \underset{j}{\operatorname{argmin}} z_{ij} (\lambda g_i d_j - \lambda g_i B - 1) \quad (8)$$

## D Proposition Proof

For each request characterized by feature  $\mathbf{x}$ , let  $K = K(\mathbf{x})$  denote the number of auto-selections. Define the prices of the  $M$  RSPs as  $X_1 = p_1(\mathbf{x}), \dots, X_M = p_M(\mathbf{x})$ , and introduce the random variables  $U_i \triangleq F_X(X_i)$  for  $i = 1, \dots, M$ , representing the Cumulative Distribution Functions (CDFs) of these prices.

Firstly,  $U_i$  is uniformly distributed over  $[0, 1]$ , because

$$P(U_i \leq u) = P(X_i \leq F_U^{-1}(u)) = F_U(F_U^{-1}(u)) = u.$$

$K$ -th order statistic is the  $K$ -th smallest value among a population. Now, we can obtain the CDF of  $K$ -th order statistic  $U_{(K)}$  among  $\{U_i\}_{i=1}^M$ . For  $U_{(K)}$  to be less or equal to  $u$ , the number of samples that are greater than  $u$  has to be less than  $M - K$ . In the case that  $U_j$  is the largest order statistic  $\leq u$ , there has to be  $j$  samples  $u$  and  $n - j$  samples larger than  $u$ . Finally, there are  $\binom{M-1}{u}$  different combinations to choose the  $n$  samples are of the  $\leq u$  kind. The corresponding CDF is:

$$F_{U_{(K)}}(u) = \sum_{j=K}^M \binom{M}{j} u^j [1 - u]^{M-j}$$

Therefore, the probability density function of  $U_{(k)}$  equals to:

$$\begin{aligned} f_{U_{(k)}}(u) &= \frac{M!}{(K-1)!(M-K)!} f_U(u) u^{K-1} [1-u]^{M-K} \\ &= \frac{M!}{(K-1)!(M-K)!} u^{K-1} [1-u]^{M-K}. \end{aligned}$$

The last equality holds since  $U \sim Uniform(0, 1)$ . That is, the  $k$ -th order statistic  $U_{(K)} = Pr(x \leq X_{(K)})$  follows the  $Beta(K, M+1-K)$ .

## E Bayesian Posterior Proof

At time  $t$ , the prior IRR distribution within cluster  $c$  for coupon  $d$  is  $Beta(\varphi | \alpha_{c,d}^{t-1}, \beta_{c,d}^{t-1})$  with density:

$$P(\varphi_t | \alpha_{c,d}^{t-1}, \beta_{c,d}^{t-1}) \propto \varphi_t^{\alpha_{c,d}^{t-1}-1} (1-\varphi_t)^{\beta_{c,d}^{t-1}-1}. \quad (9)$$

The likelihood of observing  $N_{c,d}^{in,t-1}$  In-Range outcomes out of  $N_{c,d}^{t-1}$  trials is given by

$$P(data_{t-1} | \varphi_t) \propto \varphi_t^{N_{c,d}^{in,t-1}} (1-\varphi_t)^{N_{c,d}^{t-1}-N_{c,d}^{in,t-1}}. \quad (10)$$

Applying Bayes' theorem, the posterior is

$$\begin{aligned} P(\varphi_t | data_{t-1}) &\propto P(data_{t-1} | \varphi_t) P(\varphi_t | \alpha_{c,d}^{t-1}, \beta_{c,d}^{t-1}) \\ &\propto \varphi_t^{N_{c,d}^{in,t-1} + \alpha_{c,d}^{t-1} - 1} (1-\varphi_t)^{N_{c,d}^{t-1} - N_{c,d}^{in,t-1} + \beta_{c,d}^{t-1} - 1} \\ &\propto Beta(N_{c,d}^{in,t-1} + \alpha_{c,d}^{t-1}, N_{c,d}^{t-1} - N_{c,d}^{in,t-1} + \beta_{c,d}^{t-1}). \end{aligned} \quad (11)$$
